# Supplementary material for: Few-shot Intent Classification and Slot Filling with Retrieved Examples
Source: arXiv:2104.05763 source file (2021-04-12)
Supplement: Supplementary file 2 [file d10_l10_f2.tex]

\begin{table*}[t]
\footnotesize
\begin{center}
%\resizebox{\textwidth}{!}{
\begin{tabular}{l|ccc|ccc|c}
\toprule
& \multicolumn{3}{c|}{support\_set=all} & \multicolumn{3}{c|}{support\_set=balance} & support\_set=tgt \\
\cmidrule(lr){2-4} \cmidrule(lr){5-7} \cmidrule(lr){8-8}
& tgt   & src  & avg   & tgt & src & avg   & tgt  \\ 
\midrule
\multicolumn{4}{l}{\textit{Initial BERT }}     \\
\midrule
$\texttt{Proto}^{\texttt{frz}}$  & 8.70 & 24.06 & 18.94 & - & - & - & -\\
$\texttt{Retriever}^{\texttt{frz}}$ & 3.91 & 54.96 & 37.94 & 17.38 &	16.83 & 17.01 & 27.96\\
\midrule
\multicolumn{4}{l}{\textit{Pre-train on src domain }} \\  
\midrule
\texttt{BERT fine-tune} & - & 96.51 & - & - & - & - & -\\ 
\texttt{Proto} & 76.40 & 95.70 & 89.27 & - & - & - & -\\ 
\texttt{Retriever} & 53.73 & 97.02 & 82.59 & 73.13 & 94.32 & 87.26 & 86.47\\
\texttt{Retriever  min-max} & 53.47 & 96.87 & 82.40 & 68.47 & 95.29 & 86.35 & 81.76\\
\midrule
\multicolumn{4}{l}{\textit{Fine-tune on tgt domain }} \\
\midrule 
\texttt{BERT fine-tune} & 75.57 & 50.91 & 59.13 & - & - & - & -\\
\texttt{Proto} & 76.36 & 95.06 & \textbf{88.82} & - & - & - & 86.67\\
\texttt{Retriever} & 55.20 & 97.05 & 83.10 & 74.89 & 94.57 & 88.01 & 87.74\\
\texttt{Retriever  min-max} & 55.96 & 96.92 & 83.27 & 71.09 & 95.25 & 87.19 & 83.91\\
\midrule 
\multicolumn{4}{l}{\textit{Fine-tune on tgt domain with src data}} \\ 
\midrule 
% BERT FT & 64.69 & 96.14 & 80.42 & - & - & - & -\\ 
\texttt{BERT  fine-tune} & 64.97 & 95.15 & 85.09 & - & - & - & -\\ 
\texttt{Proto} & \textbf{77.02} & 95.29 & 89.20 & - & - & - & 86.31\\
\texttt{Retriever} & 56.36 & \textbf{97.17} & 83.56 & 76.87 & 94.11 & 88.36 &  \textbf{88.18}\\
\texttt{Retriever  min-max} & 58.82 & 96.85 & 84.17 & 74.31 & 94.32 & 87.56 & 83.98\\

\bottomrule
\end{tabular}
%}
\end{center}
\caption{\label{clinc_results_10_10_2} Intent accuracy on CLINC for $n_c=10, n_i=10$ with 2-shots.}
\vspace{-1em}
\end{table*}
