# Supplementary material for: Few-shot Intent Classification and Slot Filling with Retrieved Examples
Source: arXiv:2104.05763 source file (2021-04-12)
Supplement: Supplementary file 3 [file d10_l10_f5.tex]

\begin{table*}[t]
\footnotesize
\begin{center}
%\resizebox{\textwidth}{!}{
\begin{tabular}{l|ccc|ccc|c}
\toprule
& \multicolumn{3}{c|}{support\_set=all} & \multicolumn{3}{c|}{support\_set=balance} & support\_set=tgt \\
\cmidrule(lr){2-4} \cmidrule(lr){5-7} \cmidrule(lr){8-8}
& tgt   & src  & avg   & tgt & src & avg   & tgt  \\ 
\midrule
\multicolumn{4}{l}{\textit{Initial BERT }}     \\
\midrule
$\texttt{Proto}^{\texttt{frz}}$ & 14.07 & 25.02 & 21.37 & - & - & - & -\\
$\texttt{Retriever}^{\texttt{frz}}$ & 8.24 & 54.76 & 39.25 & 22.09 & 25.29 & 24.22 & 37.93\\
\midrule
\multicolumn{4}{l}{\textit{Pre-train on src domain }} \\  
\midrule
\texttt{BERT fine-tune} & - & 96.51 & - & - & - & - & -\\ 
\texttt{Proto} & 75.02 & 95.73 & 88.83 & - & - & - & -\\ 
\texttt{Retriever} & 62.69 & \textbf{97.08} & 85.62 & 75.93 & 95.44 & 88.94 & 88.53\\
\texttt{Retriever  min-max} & 66.00 & 96.64 & 86.43 & 71.82 & 95.14 & 87.37 & 86.38\\
\midrule
\multicolumn{4}{l}{\textit{Fine-tune on tgt domain }} \\
\midrule 
\texttt{BERT fine-tune} & 78.89 & 43.91 & 55.57 & - & - & - & -\\
\texttt{Proto} & 80.44 & 95.57 & 90.53 & - & - & - & 90.35\\
\texttt{Retriever} & 66.76 & 96.95 & 86.89 & 79.20 & 95.50 & 90.07 & \textbf{91.16}\\
\texttt{Retriever  min-max} & 67.64 & 96.84 & 87.11 & 77.60 & 95.35 & 89.43 & 89.56\\
\midrule 
\multicolumn{4}{l}{\textit{Fine-tune on tgt domain with src data}} \\ 
\midrule 
% BERT FT & 64.69 & 96.14 & 80.42 & - & - & - & -\\ 
\texttt{BERT  fine-tune} & 72.00 & 95.18 & 87.45 & - & - & - & -\\ 
\texttt{Proto} & 83.33 & 94.82 & 90.99 & - & - & - & 90.22\\
\texttt{Retriever} & 69.51 & 97.04 & 87.86 & \textbf{84.95} & 95.41 & \textbf{91.92} & 90.78\\
\texttt{Retriever  min-max} & 71.35 & 96.96 & 88.42 & 81.00 & 94.55 & 90.03 & 89.82\\

\bottomrule
\end{tabular}
%}
\end{center}
\caption{\label{clinc_results_10_10_5} Intent accuracy on CLINC for $n_c=10, n_i=10$ with 5-shots.}
\vspace{-1em}
\end{table*}
