# Supplementary material for: Few-shot Intent Classification and Slot Filling with Retrieved Examples
Source: arXiv:2104.05763 source file (2021-04-12)
Supplement: Supplementary file 4 [file d5_l15_f2.tex]

\begin{table*}[t]
\footnotesize
\begin{center}
%\resizebox{\textwidth}{!}{
\begin{tabular}{l|ccc|ccc|c}
\toprule
& \multicolumn{3}{c|}{support\_set=all} & \multicolumn{3}{c|}{support\_set=balance} & support\_set=tgt \\
\cmidrule(lr){2-4} \cmidrule(lr){5-7} \cmidrule(lr){8-8}
& tgt   & src  & avg   & tgt & src & avg   & tgt  \\ 
\midrule
\multicolumn{4}{l}{\textit{Initial BERT }}     \\
\midrule
$\texttt{Proto}^{\texttt{frz}}$  & 9.39 & 16.19 & 12.79 & - & - & - & -\\
$\texttt{Retriever}^{\texttt{frz}}$ & 5.18 & 56.25 & 30.72 & 14.99 &	18.36 & 16.68 & 19.63 \\
\midrule
\multicolumn{4}{l}{\textit{Pre-train on src domain }} \\  
\midrule
\texttt{BERT fine-tune} & - & 96.87 & - & - & - & - & -
\\ 
\texttt{Proto} & 63.50 & 95.72 & 79.61 & - & - & - & -
\\ 
\texttt{Retriever} & 56.19 & \textbf{97.14} & 76.67 & 63.75 & 95.36 & 79.55 & 67.82
\\
\texttt{Retriever  min-max} & 55.88 & 96.94 & 76.41 & 60.32 & 95.50 & 77.91 & 63.60
\\
\midrule
\multicolumn{4}{l}{\textit{Fine-tune on tgt domain }} \\
\midrule 
\texttt{BERT fine-tune} & 61.91 & 77.11 & 69.51 & - & - & - & - \\
\texttt{Proto} & 66.38 & 95.72 & 81.05 & - & - & - & 70.40
\\
\texttt{Retriever} & 58.83 & 97.01 & 77.92 & 66.90 & 95.30 & 81.10 & \textbf{71.26}
\\
\texttt{Retriever  min-max} & 57.97 & 97.07 & 77.52 & 63.23 & 95.78 & 79.50 & 66.44
 \\
\midrule 
\multicolumn{4}{l}{\textit{Fine-tune on tgt domain with src data}} \\ 
\midrule 
% BERT FT &  &  &  & - & - & - & -\\ 
\texttt{BERT  fine-tune} & 60.32 & 96.16 & 78.24 & - & - & - & -
\\ 
\texttt{Proto} & 66.98 & 95.77 & \textbf{81.38} & - & - & - & 70.28
\\
\texttt{Retriever} & 59.88 & 96.96 & 78.42 & \textbf{67.23} & 94.85 & 81.04 & 70.52
\\
\texttt{Retriever  min-max} & 60.08 & 97.08 & 78.58 & 65.45 & 95.73 & 80.59 & 68.06
\\

\bottomrule
\end{tabular}
%}
\end{center}
\caption{\label{clinc_results_5_15_2} Intent accuracy on CLINC for $n_c=5, n_i=15$ with 2-shots.}
\vspace{-1em}
\end{table*}
