# Supplementary material for: Few-shot Intent Classification and Slot Filling with Retrieved Examples
Source: arXiv:2104.05763 source file (2021-04-12)
Supplement: Supplementary file 5 [file d5_l15_f5.tex]

\begin{table*}[t]
\footnotesize
\begin{center}
%\resizebox{\textwidth}{!}{
\begin{tabular}{l|ccc|ccc|c}
\toprule
& \multicolumn{3}{c|}{support\_set=all} & \multicolumn{3}{c|}{support\_set=balance} & support\_set=tgt \\
\cmidrule(lr){2-4} \cmidrule(lr){5-7} \cmidrule(lr){8-8}
& tgt   & src  & avg   & tgt & src & avg   & tgt  \\ 
\midrule
\multicolumn{4}{l}{\textit{Initial BERT }}     \\
\midrule
$\texttt{Proto}^{\texttt{frz}}$  & 15.02 & 17.58 & 16.30 & - & - & - & -\\
$\texttt{Retriever}^{\texttt{frz}}$ & 10.65 & 55.97 & 33.31 & 21.16 & 25.85 & 23.51 & 26.71\\
\midrule
\multicolumn{4}{l}{\textit{Pre-train on src domain }} \\  
\midrule
\texttt{BERT fine-tune} & - & 96.87 & - & - & - & - & -\\ 
\texttt{Proto} & 67.05 & 96.37 & 81.71 & - & - & - & -\\ 
\texttt{Retriever} & 64.19 & \textbf{97.18} & 80.69 & 68.40 & 95.85 & 82.13 & 72.02\\
\texttt{Retriever  min-max} & 61.79 & 96.71 & 79.25 & 65.11 & 95.85 & 80.48 & 68.21
\\
\midrule
\multicolumn{4}{l}{\textit{Fine-tune on tgt domain }} \\
\midrule 
\texttt{BERT fine-tune} & 69.32 & 64.76 & 67.04 & - & - & - & -
\\
\texttt{Proto} & 73.63 & 96.09 & 84.86 & - & - & - & 77.45
\\
\texttt{Retriever}& 68.65 & 97.05 & 82.85 & 74.59 & 96.24 & 85.42 & 77.96
\\
\texttt{Retriever  min-max} & 67.94 & 97.04 & 82.49 & 71.88 & 96.27 & 84.07 & 75.93
\\
\midrule 
\multicolumn{4}{l}{\textit{Fine-tune on tgt domain with src data}} \\ 
\midrule 
% BERT FT &  &  &  & - & - & - & -\\ 
\texttt{BERT  fine-tune}& 67.93 & 95.95 & 81.94 & - & - & - & -
\\ 
\texttt{Proto}& 74.43 & 95.63 & 85.03 & - & - & - & 76.61
 \\
\texttt{Retriever}& 71.51 & 96.91 & 84.21 & \textbf{76.37} & 95.81 & \textbf{86.09} & \textbf{78.62}
\\
\texttt{Retriever  min-max} & 70.50 & 96.92 & 83.71 & 73.76 & 95.79 & 84.78 & 76.65
 \\

\bottomrule
\end{tabular}
%}
\end{center}
\caption{\label{clinc_results_5_15_5} Intent accuracy on CLINC for $n_c=5, n_i=15$ with 5-shots.}
\vspace{-1em}
\end{table*}
