# Supplementary material for: Few-shot Intent Classification and Slot Filling with Retrieved Examples
Source: arXiv:2104.05763 source file (2021-04-12)
Supplement: Supplementary file 6 [file d8_l10_f2.tex]

\begin{table*}[t]
\footnotesize
\begin{center}
%\resizebox{\textwidth}{!}{
\begin{tabular}{l|ccc|ccc|c}
\toprule
& \multicolumn{3}{c|}{support\_set=all} & \multicolumn{3}{c|}{support\_set=balance} & support\_set=tgt \\
\cmidrule(lr){2-4} \cmidrule(lr){5-7} \cmidrule(lr){8-8}
& tgt   & src  & avg   & tgt & src & avg   & tgt  \\ 
\midrule
\multicolumn{4}{l}{\textit{Initial BERT }}     \\
\midrule
$\texttt{Proto}^{\texttt{frz}}$  & 7.24 & 20.99 & 14.57 & - & - & - & -\\
$\texttt{Retriever}^{\texttt{frz}}$ & 4.76 & 57.24 & 32.75 & 17.64 &	18.29 & 17.99 & 24.17 \\
\midrule
\multicolumn{4}{l}{\textit{Pre-train on src domain }} \\  
\midrule
\texttt{BERT fine-tune} & - & 96.92 & - & - & - & - & -\\ 
\texttt{Proto} & 70.59 & 94.42 & 83.30 & - & - & - & -\\ 
\texttt{Retriever} & 54.46 & \textbf{97.22} & 77.27 & 68.06 & 93.90 & 81.84 & 78.89\\
\texttt{Retriever  min-max} & 56.36 & 96.79 & 77.92 & 65.43 & 94.46 & 80.91 & 74.19\\
\midrule
\multicolumn{4}{l}{\textit{Fine-tune on tgt domain }} \\
\midrule 
\texttt{BERT fine-tune} & 68.94 & 56.41 & 62.25 & - & - & - & -\\
\texttt{Proto} & 73.19 & 94.70 & 84.66 & - & - & - & 79.83 \\
\texttt{Retriever} & 57.58 & 97.01 & 78.61 & 70.98 & 93.56 & 83.02 & \textbf{80.35} \\
\texttt{Retriever  min-max} & 58.71 & 96.89 & 79.07 & 68.71 & 94.64 & 82.54 & 76.51\\
\midrule 
\multicolumn{4}{l}{\textit{Fine-tune on tgt domain with src data}} \\ 
\midrule 
% BERT FT &  &  &  & - & - & - & -\\ 
\texttt{BERT  fine-tune} & 61.53 & 95.10 & 79.43 & - & - & - & -\\ 
\texttt{Proto} & \textbf{73.57} & 94.59 & \textbf{84.78} & - & - & - & 80.08\\
\texttt{Retriever} & 59.06 & 97.07 & 79.33 & 72.33 & 93.11 & 83.42 & 80.14\\
\texttt{Retriever  min-max} & 60.49 & 96.89 & 79.91 & 70.92 & 94.68 & 83.59 & 79.21 \\

\bottomrule
\end{tabular}
%}
\end{center}
\caption{\label{clinc_results_8_10_2} Intent accuracy on CLINC for $n_c=8, n_i=10$ with 2-shots.}
\vspace{-1em}
\end{table*}
