# Supplementary material for: Few-shot Intent Classification and Slot Filling with Retrieved Examples
Source: arXiv:2104.05763 source file (2021-04-12)
Supplement: Supplementary file 7 [file d8_l10_f5.tex]

\begin{table*}[t]
\footnotesize
\begin{center}
%\resizebox{\textwidth}{!}{
\begin{tabular}{l|ccc|ccc|c}
\toprule
& \multicolumn{3}{c|}{support\_set=all} & \multicolumn{3}{c|}{support\_set=balance} & support\_set=tgt \\
\cmidrule(lr){2-4} \cmidrule(lr){5-7} \cmidrule(lr){8-8}
& tgt   & src  & avg   & tgt & src & avg   & tgt  \\ 
\midrule
\multicolumn{4}{l}{\textit{Initial BERT }}     \\
\midrule
$\texttt{Proto}^{\texttt{frz}}$  & 12.57 & 21.67 & 17.42 & - & - & - & -\\
$\texttt{Retriever}^{\texttt{frz}}$ & 9.46 & 56.96 & 34.79 & 23.37 & 25.87 & 24.70 & 32.72 \\
\midrule
\multicolumn{4}{l}{\textit{Pre-train on src domain }} \\  
\midrule
\texttt{BERT fine-tune} &- & 96.92 & - & - & - & - & -\\ 
\texttt{Proto} & 73.17 & 94.96 & 84.79 & - & - & - & -\\ 
\texttt{Retriever} & 66.56 & 96.76 & 82.67 & 76.56 & 94.99 & 86.39 & 83.72 \\
\texttt{Retriever  min-max} & 66.08 & 96.64 & 82.38 & 73.14 & 95.13 & 84.87 & 79.52 \\
\midrule
\multicolumn{4}{l}{\textit{Fine-tune on tgt domain }} \\
\midrule 
\texttt{BERT fine-tune} & 76.92 & 44.17 & 59.45 & - & - & - & -\\
\texttt{Proto} & 77.53 & 94.88 & 86.78 & - & - & - & 85.21\\
\texttt{Retriever} & 68.35 & \textbf{97.11} & 83.69 & 77.54 & 95.67 & 87.21 & 85.72\\
\texttt{Retriever  min-max} & 70.65 & 96.76 & 84.58 & 76.74 & 94.90 & 86.43 & 85.41\\
\midrule 
\multicolumn{4}{l}{\textit{Fine-tune on tgt domain with src data}} \\ 
\midrule 
% BERT FT &  &  &  & - & - & - & -\\ 
\texttt{BERT  fine-tune} & 70.48 & 95.11 & 83.61 & - & - & - & -\\ 
\texttt{Proto} & 79.89 & 94.32 & 87.59 & - & - & - & 85.41 \\
\texttt{Retriever} & 71.46 & 96.88 & 85.02 & \textbf{79.90} & 94.61 & \textbf{87.75} & \textbf{89.67}\\
\texttt{Retriever  min-max} & 71.73 & 96.86 & 85.13 & 78.43 & 95.31 & 87.43 & 85.32\\

\bottomrule
\end{tabular}
%}
\end{center}
\caption{\label{clinc_results_8_10_5} Intent accuracy on CLINC for $n_c=8, n_i=10$ with 5-shots.}
\vspace{-1em}
\end{table*}
